# Supplementary material for: Multi-modality Meets Re-learning: Mitigating Negative Transfer in Sequential Recommendation
Source: arXiv:2309.10195 source file (2023-09-20)
Supplement: Supplementary file 1 [file appendix.pdf]

## APPENDIX A

### REPRODUCIBILITY

We implement ANT in Python 3.9.13 with PyTorch 1.10.2<sup>5</sup> and PyTorch Lightning 1.7.7<sup>6</sup>. Following UniSRec and SASRec, we set the number of self-attention layers and the number of attention heads in each layer as 2, and the dimension for item embeddings as 256 for ANT and all the baseline methods if applicable. We also use the cross entropy loss for ANT and all the baseline methods to enable a fair comparison. Following UniSRec, in ANT, we set the scaling hyper-parameters  $\tau$  (Equation 13) as 0.07; set the number of projection heads in embedding transformation  $n_h$  as 8; and use Adam optimizer with learning rate  $1e-3$  on all the datasets. In ANT, we also set the dimension of price embeddings  $d_p$  as 64; use 50,000 as the frequency coefficient  $\omega$  (Equation 3); and normalize the item prices to be in the range of  $[0, 100]$ . Considering the memory limits in GPUs, we use batch optimization during pre-training and adaptation, and set the batch size as 2,048 following UniSRec. For ANT and all the baseline methods, we initialize all the learnable parameters using the default initialization methods in PyTorch. For NOVA and SASRec++, we search the dimension of item embeddings  $d$  from  $\{64, 128, 256\}$ . In ANT, we search the coefficient of modality interaction embeddings  $\beta$  (Equation 9) from  $\{0.1, 0.3, 0.5, 0.7\}$ . For UniSRec, we use the hyper-parameters reported by the authors in all the datasets. For NPE, SASRec, BERT4Rec, FDSA and S3-Rec, following UniSRec, we search  $d$  and the learning rate  $lr$  from  $\{64, 128, 300\}$  and  $\{3e-4, 1e-3, 3e-3, 1e-2\}$ , respectively. Table A1 presents the best-performing hyper-parameters in ANT, ANT<sub>e</sub> and all the baseline methods except for UniSRec on the five datasets. We refer the audience of interest to the UniSRec’s GitHub<sup>7</sup> for the hyper-parameters used in UniSRec.

5. <https://pytorch.org/>

6. <https://www.pytorchlightning.ai/>

7. <https://github.com/RUCAIBox/UniSRec>

TABLE A1: Best-performing Hyper-parameters in ANT, ANT<sub>e</sub> and Baseline Methods

| Dataset     | NPE |      | SASRec |      | BERT4Rec |      | FDSA |      | S3-Rec |      | NOVA | SASRec++ | ANT     | ANT <sub>e</sub> |
|-------------|-----|------|--------|------|----------|------|------|------|--------|------|------|----------|---------|------------------|
|             | $d$ | $lr$ | $d$    | $lr$ | $d$      | $lr$ | $d$  | $lr$ | $d$    | $lr$ | $d$  | $d$      | $\beta$ | $\beta$          |
| Scientific  | 300 | 3e-3 | 128    | 1e-3 | 128      | 1e-2 | 64   | 3e-3 | 300    | 3e-3 | 256  | 256      | 0.1     | 0.1              |
| Pantry      | 128 | 3e-3 | 300    | 3e-4 | 300      | 3e-3 | 64   | 1e-3 | 300    | 1e-3 | 256  | 256      | 0.3     | 0.5              |
| Instruments | 128 | 1e-3 | 300    | 3e-4 | 300      | 3e-4 | 128  | 3e-3 | 300    | 1e-3 | 128  | 256      | 0.7     | 0.1              |
| Arts        | 128 | 1e-3 | 300    | 3e-4 | 300      | 3e-4 | 128  | 3e-3 | 300    | 3e-3 | 256  | 256      | 0.7     | 0.1              |
| Office      | 128 | 1e-3 | 300    | 3e-4 | 300      | 3e-4 | 128  | 1e-3 | 300    | 3e-3 | 128  | 256      | 0.5     | 0.1              |

This table presents the best-performing hyper-parameters of ANT, ANT<sub>e</sub> and all the baseline methods except for UniSRec on the five datasets.
